# Supplementary material for: Unified Shape and SVBRDF Recovery using Differentiable Monte Carlo Rendering
Source: arXiv:2103.15208 source file (2021-06-25)
Supplement: Supplementary file 2 [file supp_setup.tex]

\section{Acquisition setup}
\label{sec:setup}
To produce the reconstruction results of real-world objects in the paper and Figure~\ref{fig:main2_supp}, our method takes as input multi-view photos that can be captured using a camera with flashlight, or with a consumer-level RGBD sensor.
%In the later case, we can also utilize the depth information from RGBD sensor to accelarate the optimization process.
%
\iffalse
	\begin{figure}[htp]
		\centering
	 
		\addtolength{\tabcolsep}{-4.5pt}
		\begin{tabular}{cc}
			{\scriptsize iPhone} & {\scriptsize Microsoft Azure Kinect}\\
			\includegraphics[height=1.65in]{setup/capture_iphone.jpg} &
			\includegraphics[height=1.65in]{setup/capture_sensor.jpg}
		\end{tabular}
	    \caption{Multi-view acquisition setup. Our pipeline takes as input a set of photos captured by a collocated camera-light setup, which is commonly found on mobile phones or easily built on a consumer-level RGBD sensor, both with a collocated small LED light.}
	    \label{fig:setup}
	    %\vspace*{-1.5\baselineskip}%
	\end{figure}
\else
	\begin{center}
		\addtolength{\tabcolsep}{-4.5pt}
		\begin{tabular}{cc}
			{\scriptsize iPhone} & {\scriptsize Microsoft Azure Kinect}\\
			\includegraphics[height=1.65in]{setup/capture_iphone.jpg} &
			\includegraphics[height=1.65in]{setup/capture_sensor.jpg}
		\end{tabular}
	\end{center}
\fi
