# Supplementary material for: Unified Shape and SVBRDF Recovery using Differentiable Monte Carlo Rendering
Source: arXiv:2103.15208 source file (2021-06-25)
Supplement: Supplementary file 3 [file supp_tab_stages.tex]

\begin{table}[htp]
	\centering
	\small
	\caption{\label{tab:supp_stages}
		\textbf{Number of stages and iterations per stage.} We report the number of stages in coarse-to-fine pipeline, and number of Adam iterations in each stage for both synthetic and real data.
	}
	\vspace{1em}
	\addtolength{\tabcolsep}{-3.5pt}
	\begin{tabular}{lcccccccc} 
		\toprule
		        &  Kitty & Duck & Bell & Pig  & Pony & Chime & Nefertiti & Buddha \\ 
		Stage 1 &  500   & 500  & 500  & 500  & 500  &  500  & 500       & 500    \\
		Stage 2 &  500   & 500  & 1000 & 1000 & 1000 & 1000  & 1000      & 1000   \\
		Stage 3 &  N/A   & N/A  & 500  & 500  & N/A  & 1000  & 1000      & 1000   \\
		Stage 4 &  N/A   & N/A  & N/A  & N/A  & N/A  &  500  & 500       & 500   \\
		\bottomrule
	\end{tabular}%
\end{table}
